# Supplementary material for: Bidirectional electro-optic conversion reaching 1% efficiency with thin-film lithium niobate
Source: arXiv:2012.14909 ancillary file (2021-01-01)
Supplement: Supplementary file 1 [file Supplementary_for_Conversion.pdf]

# Bidirectional electro-optic conversion reaching 1% efficiency with thin-film lithium niobate

YUNTAO XU[1,†], AYED AL SAYEM[1,†], LINRAN FAN[2], SIHAO WANG[1], RISHENG CHENG[1], CHANGLING-ZOU[1], WEI FU[1], LIKAI YANG[1], MINGRUI XU[1], AND HONG X. TANG[1,*]

[1] *Department of Electrical Engineering, Yale University, New Haven, CT 06511, USA*
[2] *James C. Wyant College of Optical Sciences, The University of Arizona, Tucson, Arizona 85721, USA*
[*] *Corresponding author: hong.tang@yale.edu*
[†] *These authors contributed equally to this Letter.*

## 1. THE VACUUM EO COUPLING RATE

In a general cavity EO system, the vacuum coupling rate, $g_{eo}$ can be expressed as [1],

$$\hbar g_{eo} = \frac{\int (\varepsilon_{a,i}\varepsilon_{b,j}r_{ijk}) \cdot (u_{a,i}u^*_{b,j}u_{c,k})dxdydz}{\sqrt{2\varepsilon_0}U_a U_b U_c}. \tag{S1}$$

Here $\varepsilon_{l,i}$ and $u_{l,i}$ ($l \in \{a,b,c\}, i \in \{x,y,z\}$) denote the relative permittivity and electric field components respectively and $r_{ijk}$ is the electro-optic coefficient of the nonlinear material. $U_l = \sqrt{2\int \varepsilon_{l,i}u_{l,i}u^*_{l,i}dxdydz/\hbar\omega_l}$ is the normalizing factor, where $\omega_l$ denote the resonance frequency. In our TFLN double ring design, the two optical mode profiles are identical and the microwave electric field in LN can be approximated as uniform, the expression could be simplified as

$$g_{eo} \approx \frac{3}{16} n^2_{\text{eff}} r_{33}\omega_a \frac{u_{c,r}}{U_c}. \tag{S2}$$

Here $u_{c,r}$ denotes the radial component of microwave electric field, $n_{\text{eff}} = [2n_o^2 n_e^2/(n_o^2 + n_e^2)]^{1/2}$ is the effective index of the fundamental TE mode in the optical cavity and $r_{33} \approx 30\text{pm/V}$ is the electro-optic coefficient of LN. Considering the optical energy is distributed between two rings, we have a factor of 1/2 here; an additional factor of 3/8 comes from the misalignment of radial optical TE field with the z-axis of x-cut LN film. Using finite element method (FEM) simulation and utilizing Eqn. S2, the calculated vacuum coupling rate, $g_{eo}$ is 1.5 kHz.

## 2. DEVICE PARAMETERS

Shown in Table S1 are the detailed device characteristics of optical and microwave modes used during conversion characterization.

**Table S1.** Device parameters

| | frequency $\omega/2\pi$ | total loss rate $\kappa/2\pi$ | external loss rate $\kappa_{ex}/2\pi$ |
|---|---|---|---|
| Pump mode $a$ | 193.34 THz (CW)<br>192.83 THz (pulsed) | 301 MHz (CW)<br>380 MHz (pulsed) | 109 MHz (CW)<br>124 MHz (pulsed) |
| Signal mode $b$ | 193.35 THz (CW)<br>192.84 THz (pulsed) | 173 MHz (CW)<br>280 MHz (pulsed) | 33 MHz (CW)<br>52 MHz (pulsed) |
| MW mode $c$ | 7.836 GHz | 9.06 MHz | 3.22 MHz |

## REFERENCES

1. L. Fan, C.-L. Zou, R. Cheng, X. Guo, X. Han, Z. Gong, S. Wang, and H. X. Tang, "Superconducting cavity electro-optics: a platform for coherent photon conversion between superconducting and photonic circuits," Sci. Adv. **4**, eaar4994 (2018).
